# Supplementary material for: GRILL: Grounded Vision-language Pre-training via Aligning Text and Image Regions
Source: arXiv:2305.14676 source file (2023-05-24)
Supplement: Supplementary file 1 [file 090appendix.tex]

% \begin{table}[tb!]
% \centering
% \caption{\textbf{Model architectures.} }
% \resizebox{0.98\linewidth}{!}{
% \begin{tabular}[t]{L{3cm}|C{2.5cm}C{2.5cm}}
% \toprule
%     \textbf{Hyperparameter}  &\textbf{\method$_{base}$}     &\textbf{\method$_{large}$} \\
% \midrule
% \# Layers &12+12   &24+24          \\
% Hidden dimension &768   &1,024    \\
% FF hidden size &3,072   &4,096    \\
% \# Attention head  &12   &16   \\
% Attention head size &64  &64    \\
% \bottomrule
% \end{tabular}}
% \label{tab:modelpara}
% \end{table}

% \section{Model Architectures}
% Table~\ref{tab:modelpara} shows model parameters in our model, \method. \method$_{base}$ and  \method$_{large}$ is based on VL-T5~\cite{cho2021unifying} and T5~\cite{raffel2019exploring}, respectively.

\section{Detailed Model Architecture}
\label{append:arch}
We adopt an encoder-decoder architecture~\citep{vaswani2017attention} to encode visual and text inputs to generate target text.
We represent an input image with a sequence of image patches by a vision transformer~\citep{dosovitskiy2020image,liu2021swin}. 
We adopt Swin transformer (Swin-B)~\citep{liu2021swin} as our vision transformer.
The numbers of layers in our transformer encoder and decoder are 12 and 12, respectively, Hidden dimension is 768, the number of attention heads is 12 and the attention head size is 64.
We train the model parameters $\theta$ by minimizing the negative log-likelihood of target text $y$ tokens given input text $x$ and image $v$:
\begin{equation}
\label{loss}
L_\theta = -\sum_{i=1}^{|y|} \log P_\theta (y_i | y_{<i}, x, v).
\end{equation}

% We adopt an encoder-decoder architecture~\citep{vaswani2017attention} to encode visual and text inputs to generate target text.
% We represent an input image with a sequence of image patches by a vision transformer~\citep{dosovitskiy2020image,liu2021swin}. 
% We adopt Swin transformer (Swin-B)~\citep{liu2021swin} as our vision transformer.
% It first splits an image into non-overlapping patches and linearly embeds all patches. Then, these patches are passed to the transformer encoder layers, yielding $\{v_1, ..., v_m \}$. For an image of resolution of $224 \times 224$ and patch size of $32 \times 32$, we have $m = 49$.
% We assume that $v_i$ encodes the information of the corresponding patch $p_i$. 
% Therefore, we represent a visual concept (object or region) $V_j$ that corresponds to a set of patches by aggregating information among the patches as shown in Figure~\ref{fig:illust}.
% In addition, the entire patch representations are fed into the encoder by appending them to the text to encode the whole image.
% Then the transformer decoder outputs the target text.
% We train the model parameters $\theta$ by minimizing the negative log-likelihood of target text $y$ tokens given input text $x$ and image $v$:
% \begin{equation}
% \label{loss}
% L_\theta = -\sum_{i=1}^{|y|} \log P_\theta (y_i | y_{<i}, x, v).
% \end{equation}
% \section{Details of Creating Negative Examples}

\section{Details of Pre-training Data}
To pre-train \method, we collect image-caption data from MS COCO~\citep{lin2014microsoft,chen2015microsoft} and Visual Genome (VG)~\citep{krishna2017visual}.
The pre-training datasets contain 6M image-text pairs and 180K distinct images.
MS-COCO has 123K images and 617K captions while VG has 108K images and 5.30M captions. They share 51K images in common.
We obtained 1.8 object-word alignments per image-caption pair on average.

\section{Fully Fine-tuning Results}
We test our model on the fully-supervised setting in Table~\ref{tab:full}.
We used test sets for RefCOCOg, Flickr30k-entities, NLVR2, SNLI-VE, Flickr30k, the val set for VCR, and test-std for VQAv2 for evaluation.
We report Q $\rightarrow$ AR for VCR.
We quote the VCR results of VL-T5 and UNITER pre-trained with stage 1 for a fair comparison~\cite{cho2021unifying,chen2019uniter}.
% VL-T5 only stage 1. VCR val
Our model underperforms other competitors on many tasks, especially classification tasks, VCR, RefCOCOg, Flickr30k-entities, NLVR2, and SNLI-VE.
We conjecture that our discriminative objective require the model to generate binary decisions, ``true'' and ``false'', which possibly is limited in multi-class classification tasks. 
However, it is challenging to design a classification head or generations for multiple classes without knowing the number of classes.
We leave the sophisticated design for future work.
% These tasks mul

\begin{table*}[!t]
	\centering
	\small
	\resizebox{\textwidth}{!}{
		\begin{tabular}{l|ccccccccc}
            \toprule
           \multirow{2}{*}{\textbf{Method} } &   \multicolumn{1}{c}{\textbf{VCR}} & \multicolumn{1}{c}{\textbf{RefCOCOg}} &  \multicolumn{3}{c}{\textbf{Flickr30k-entities}}  & \multicolumn{1}{c}{\textbf{NLVR2}} & \multicolumn{1}{c}{\textbf{SNLI-VE}} & \multicolumn{1}{c}{\textbf{VQAv2}} & \multicolumn{1}{c}{\textbf{Flickr30k}}\\
            \cmidrule(lr){2-2} \cmidrule(lr){3-3}     \cmidrule(lr){4-6} \cmidrule(lr){7-7}  \cmidrule(lr){8-8} \cmidrule(lr){9-9} \cmidrule(lr){10-10} 
            &  Q $\rightarrow$ AR & Acc & R@1 & R@5 & R@10 & Acc & Acc & Acc & CIDEr \\
            \midrule
            Random              & 6.3   & 19.0  & 6.5   & 27.7  & 47.8  & 50.0  & 33.3  & 0.0     & - \\
            UNITER$_{base}$    & 54.9 & 74.51 & - & - &-  & 77.85 & 78.28 & 72.91 & - \\
            UNITER$_{large}$    & - & 75.77 & - & - &-  & 79.98 & 79.38 & 73.82 & - \\
            VL-T5               & 54.7 & 71.3    & - & - & - & 73.6 & - & 70.3 & - \\
            % VL-T5               & 224M  & 29.7  & 28.0  & 8.7   & 27.3  & 23.6  & 56.4  & 70.2  & -     & 27.9 \\
            % VL-T5 (with prompt) & 224M  &       &       &       &\bf 56.9&\bf 51.0 & 72.8& 78.6 & -     & - \\
            % FewVLM$_{base}$     & 224M  & & & & & & & & & & & \\
            % FewVLM$_{large}$    & 740M  & & & & & & & & & & & \\
            % Oscar$_{large}$     & -     & -     & -     & -     & -     & -     & -     & -     & - \\
            MDETR-ENB3          & - & 83.31 & 84.0 & 93.8 & 95.6 & - & - & - & - \\
            GLIP-L              & - & - & 87.1 & 96.9 & 98.1 & - & - & - & -\\
            Unified VLP         & - & - & - & - & - & - & - & 70.7 & 67.4 \\
            % Flamingo            & - & - & - & - & - & - & - & - & - & 67.6 & 75.4 \\ 
            \midrule
            \methodn            &50.64   & 55.65    & 42.89    & 76.59 & 83.88 & 68.42 & 77.05 & 70.21 & 67.75 \\
            % \methodn$_{large}$  & 825M  & 41.1  & 40.7  & 17.3  & 46.6  & 25.6  & 57.5  & 71.8  & 56.7  & 49.9  & 49.1    & 37.5 \\
            \bottomrule
        \end{tabular}
	}
	\caption{\textbf{Fully fine-tuning results.} 
 % $^\dagger$We report zero-shot results since their model is already trained on the Flickr30k-entities. Flamingo used 16 examples in this setup. 
	}
	\label{tab:full}
\end{table*}

\begin{figure}[tb!]
    \centering
    \subfloat[SNLI-VE]{\includegraphics[width=0.45\columnwidth]{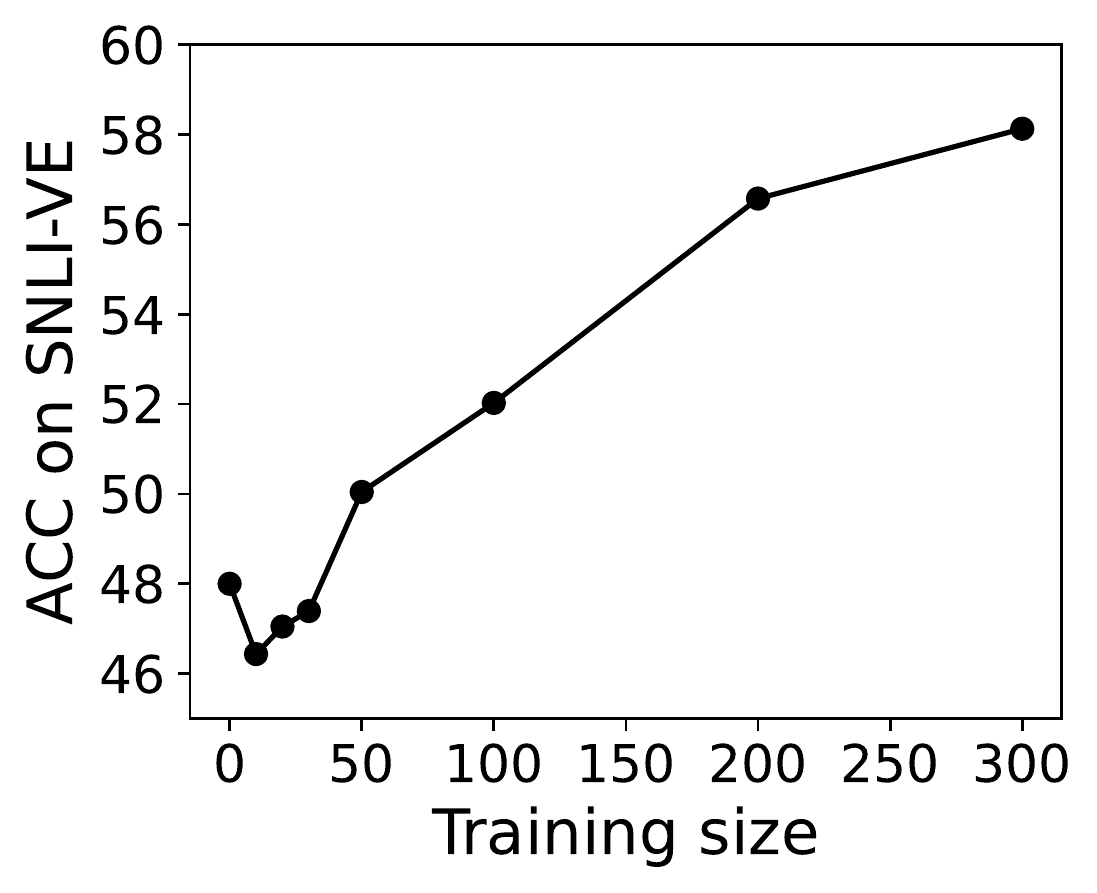}}
    \quad
    \subfloat[NLVR2]{\includegraphics[width=0.45\columnwidth]{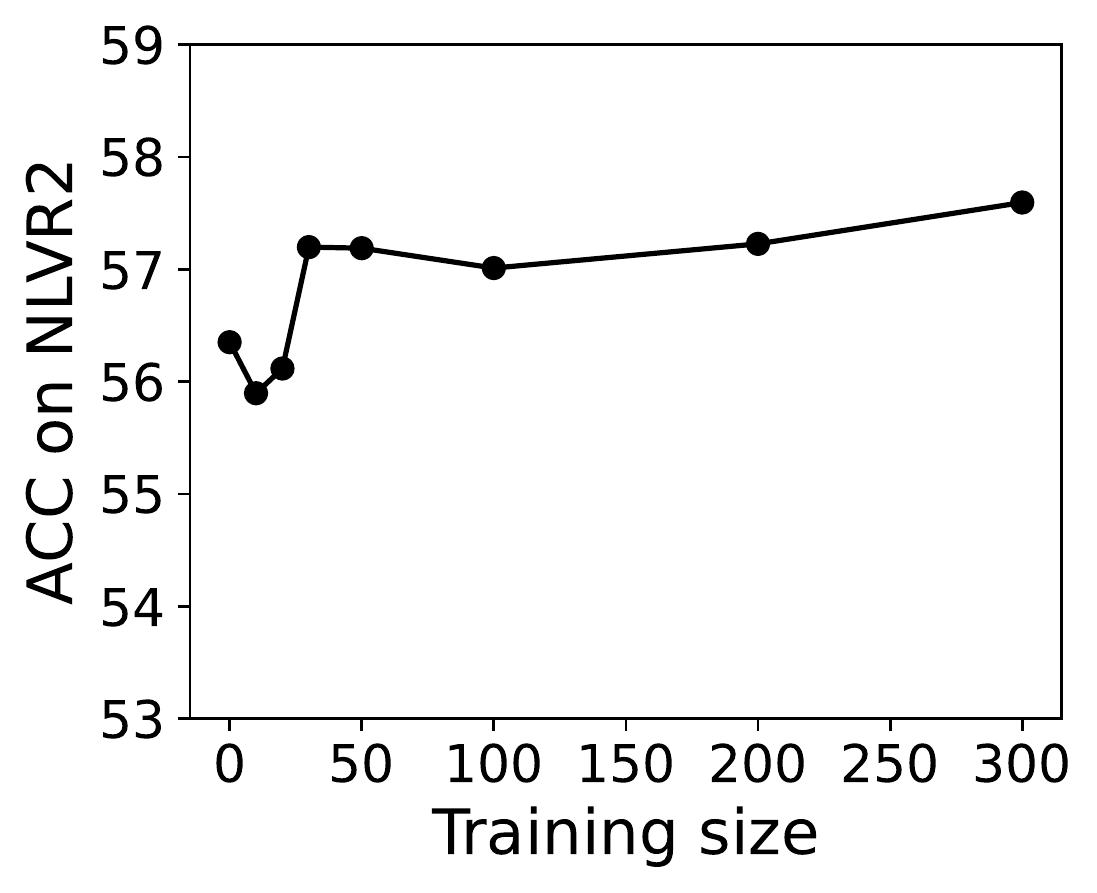} }
    \caption{\textbf{Results with different training sizes.} We evaluate our model with different training sizes.}
    \label{fig:size}
\end{figure}

\section{Ablations on Different Training Sizes}
We evaluate our model with different training sizes on SNLI-VE and NLVR2 datasets in Fig.~\ref{fig:size}.
We observe that the model performance is increasing with larger training sizes on the datasets.

% \section{Pre-training Data}
% \para{Object-word alignments.}
% \wj{need to elaborate CLIP}
% In the last step, we find alignments between object bounding boxes and words $\{(o_i, w_j)\}$ given the alignments between tags and words $\{(l_i, w_j)\}$ and an object list $\{(o_1, l_1), ..., (o_m, l_m)\}$. 
% % Thus, we get $\{(o_i,l_i,w_j) \}$.
% We simply find the object-word alignments since each tag is mapped to each bounding box, yielding $\{(o_i,l_i,w_j) \}$.
% However, note that some object bounding boxes share the same object tag; thus the alignments can include noisy correspondence between object boxes and words.
% % it is important to find the most plausible alignment.
% We run CLIP~\cite{radford2021learning} between aligned words and objects to find the most plausible alignment.  
% To consider contextualized word representations in a caption, we use a window that includes the word we are interested in to find alignments. \wj{need to improve language here}

% \section{Downstream Tasks}
% \wj{statistics}

% We use Karpathy split~\citep{karpathy2015deep} for Flickr30k, which re-splits train and val images into 29,000 / 1,014 / 1,000 for train / validation / test.
% \wj{refer to vlt5 and flamingo for dataset table}

% \begin{figure}[tb!]
%     \centering
%     {\includegraphics[width=1\linewidth]{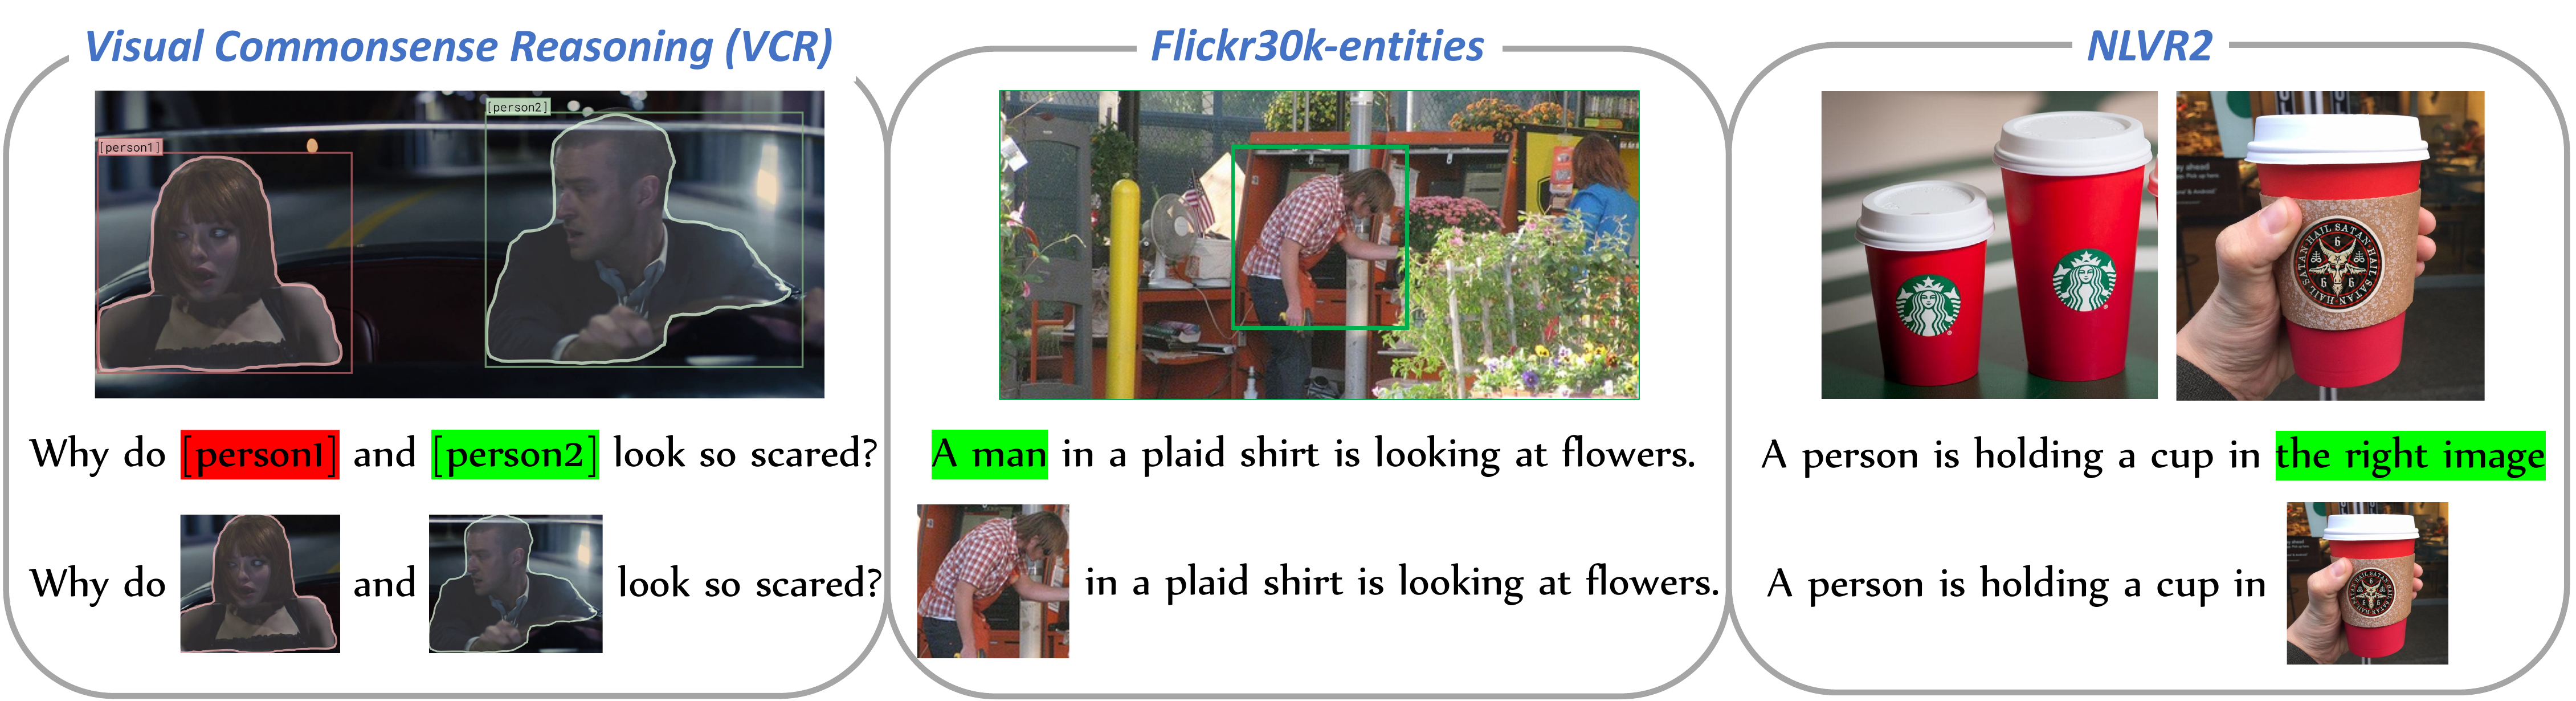}}
%     \caption{\textbf{Example inputs for inference.} We resolve the grounding by replacing referring words with corresponding bounding boxes.  
%     }
%     \label{fig:example}
% \end{figure}

% \wj{need to write how to implement VL-T5 on flickr30k entities, VQA}
